# Supplementary material for: LLM-AutoDiff: Auto-Differentiate Any LLM Workflow
Source: arXiv:2501.16673 source file (2025-01-30)
Supplement: Supplementary file 1 [file appendix_ex.tex]

\section{Appendix}

\subsection{Meta Prompts}

\minisection{Meta Prompts for backward engine} \label{appendix: meta_prompts_backward_engine}

All these prompts are located in directory \texttt{adalflow/adalflow/optim/text\_grad/backend\_engine\_prompt.py}.

% \minisection{Meta prompts in the lossComponent to get gradients to previous outputs} \label{appendix: loss_component_meta_prompts}

% Meta prompts with two subprompts: \texttt{conversation\_sec} and \texttt{objective\_instruction\_sec} are used in the \texttt{lossComponent} to get gradients to previous outputs.
The general template for the backward engine.

\begin{lstlisting}[
    basicstyle=\ttfamily\small,
    breaklines=true,
    language=Python,
    keywordstyle=\color{blue}\bfseries,
    stringstyle=\color{orange},
    commentstyle=\color{green!50!black},
    frame=single,
    showstringspaces=false,
    tabsize=4,
    numbers=left,
    numberstyle=\tiny\color{gray}
]
FEEDBACK_ENGINE_TEMPLATE = r"""
<START_OF_SYSTEM_PROMPT>
You are the feedback engine in an optimization system.

Your role: Provide intelligent and creative feedback for the variable enclosed in <VARIABLE></VARIABLE> tags, based on the objective specified in <OBJECTIVE_FUNCTION></OBJECTIVE_FUNCTION> tags.
1. Focus on the downstream OBJECTIVE without proposing new versions of the variable.
2. Feedback examples: "Since language models have the X failure mode...", "Adding X can fix this error because...", "Removing X can improve the objective function because...", "Changing X to Y would fix the mistake..."
3. Consider the variable in the context of its peers if provided.
Remember:
Be concise, critical, and direct.
<END_OF_SYSTEM_PROMPT>
<CONVERSATION>
{{conversation_sec}}
</CONVERSATION>
{{objective_instruction_sec}}
"""
\end{lstlisting}

\paragraph{Loss Component }
For the loss component, it is the last node with an evaluation function. The definition of those two subprompts is as follows:

\begin{lstlisting}[
    basicstyle=\ttfamily\small,
    breaklines=true,
    language=Python,
    keywordstyle=\color{blue}\bfseries,
    stringstyle=\color{orange},
    commentstyle=\color{green!50!black},
    frame=single,
    showstringspaces=false,
    tabsize=4,
    numbers=left,
    numberstyle=\tiny\color{gray}]
OBJECTIVE_INSTRUCTION_BASE = r"""
<OBJECTIVE_FUNCTION>
Your only goal is to clearly states how it obtained the "<OUTPUTS/SCORE>".
Your only goal is to clearly states how it obtained the "<OUTPUTS/SCORE>".
Especially when the score is low.
Be CONCISE.
If you have enough context, add a more specific feedback on how it failed.
</OBJECTIVE_FUNCTION>"""
\end{lstlisting}

\begin{lstlisting}[
    basicstyle=\ttfamily\small,
    breaklines=true,
    language=Python,
    keywordstyle=\color{blue}\bfseries,
    stringstyle=\color{orange},
    commentstyle=\color{green!50!black},
    frame=single,
    showstringspaces=false,
    tabsize=4,
    numbers=left,
    numberstyle=\tiny\color{gray}
]
CONVERSATION_START_INSTRUCTION_BASE = r"""
{{variable_and_peers_info}}

Here is an evaluation of the variable using a language model:
{{conversation_str}}
"""
\end{lstlisting}

For the \texttt{conversation\_sec} placeholder, the following template is used:

\begin{lstlisting}[
    basicstyle=\ttfamily\small,
    breaklines=true,
    language=Python,
    keywordstyle=\color{blue}\bfseries,
    stringstyle=\color{orange},
    commentstyle=\color{green!50!black},
    frame=single,
    showstringspaces=false,
    tabsize=4,
    numbers=left,
    numberstyle=\tiny\color{gray}
]
### Variable to get feedback on, often it is pred in the loss component
LOSS_CONVERSATION_START_INSTRUCTION_STRING_FN = r"""
TARGET VARIABLE:
<NAME> {{variable_name}} </NAME>
<ROLE> {{variable_desc}} </ROLE>
<VARIABLE> {{variable_value}} </VARIABLE>
{{conversation_str}}
"""

###  Loss/Score Information  ###
LOSS_CONVERSATION_TEMPLATE_STRING = r"""
The variable is passed to the eval function and compared with a target/ground truth value.

<EVAL_FUNC_DESCRIPTION>: {{eval_fn_desc}}
<INPUTS>: {{input_str}}
<OUTPUTS/SCORE>: {{response_value}}
{% if metadata %}
Note: {{metadata}}
{% endif %}"""
\end{lstlisting}   

\paragraph{Intermediate Generator Component}
For the intermediate generator output, the following template is used:

\begin{lstlisting}[
    basicstyle=\ttfamily\small,
    breaklines=true,
    language=Python,
    keywordstyle=\color{blue}\bfseries,
    stringstyle=\color{orange},
    commentstyle=\color{green!50!black},
    frame=single,
    showstringspaces=false,
    tabsize=4,
    numbers=left,
    numberstyle=\tiny\color{gray}
]

######################################
# LLM as gradComponent
######################################
# When the parameter has a gradient, it is the continuation of the backpropagation chain, a layer in the models
CONVERSATION_START_INSTRUCTION_CHAIN = r"""
{{variable_and_peers_info}}

Here is a conversation with a language model (LM):
{{conversation_str}}
"""

OBJECTIVE_INSTRUCTION_CHAIN = r"""
This conversation is part of a larger system. The <LM_OUTPUT> was later used as {{response_desc}}.
<OBJECTIVE_FUNCTION>
Your goal is to give feedback to the variable with the LLM_OUTPUT: {{response_gradient}}
{% if instruction_to_backward_engine %}
Note: {{instruction_to_backward_engine}}
{% endif %}
</OBJECTIVE_FUNCTION>"""

###  Backward engine: user prompt
# First part to provide context of LLM as gradComponent
# The target variable is used as either input or a task instruction to a language model (LM):
# replace the "The target variable is used as either input or a task instruction to a language model (LM):" with the {{variable_desc}}
LLM_CONVERSATION_TEMPLATE = r"""
NAME: {{variable_name}}
Description: {{variable_desc}}

LM_INPUT: {{input_value}}
LM_OUTPUT: {{llm_output}}"""


VARIABLE_AND_PEERS_INFO = r"""
<START_OF_VARIABLE_DESC>
{{variable.name}}
<TYPE> {{variable.param_type}} </TYPE>
<ROLE> {{variable.role_desc}} </ROLE>
<VARIABLE> {{variable.data}} </VARIABLE>
<END_OF_VARIABLE_DESC>
{% if peers %}
<VARIBLE_PEERS>
The variable is used together with the these peer variables to instruct the language model:
{% for peer in peers %}
{{loop.index}}.
PEER_NAME: {{peer.name}},
PEER_TYPE: {{peer.param_type}},
PEER_ROLE: {{peer.role_desc}}
WILL_BE_OPTIMIZED: {{peer.requires_opt}}
{% if peer.data %}
PEER_VARIABLE: {{peer.data}}
{% else %}
PEER_VARIABLE: EMPTY
{% endif %}
{% endfor %}
</VARIBLE_PEERS>
{% endif %}
"""
\end{lstlisting}

\minisection{Meta prompts for the optimizer}

The relevant meta prompts located in \texttt{adalflow/\allowbreak adalflow/\allowbreak optim/\allowbreak text\_grad/\allowbreak tgd\_optimizer.py}. 
are as follows:

\begin{lstlisting}[
    basicstyle=\ttfamily\small,
    breaklines=true,
    language=Python,
    keywordstyle=\color{blue}\bfseries,
    stringstyle=\color{orange},
    commentstyle=\color{green!50!black},
    frame=single,
    showstringspaces=false,
    tabsize=4,
    numbers=left,
    numberstyle=\tiny\color{gray}
]
TEXT_GRAD_DESC_TEMPLATE = r"""<START_OF_SYSTEM_PROMPT>
{{optimizer_system_prompt}}
<END_OF_SYSTEM_PROMPT>
<START_OF_USER_MESSAGE>
{#Variable and feedback#}
{{variable_and_peers_info}}
{# ORPO past history #}
{% if past_history %}
<START_OF_HISTORY_PERFORMANCE>
Here are the past iterations of this variable along with the validation score.
{% for history in past_history %}
{{loop.index}}. {{history}}
{% endfor %}
IMPORTANT: Your goal is to generate new variable values that score higher than all previous iterations.
<END_OF_HISTORY_PERFORMANCE>
{% endif %}
Here are the context and feedback for the variable:
<START_OF_CONTEXT_FEEDBACK>
{{variable_grad}}
<END_OF_CONTEXT_FEEDBACK>
{# Momentum #}
{% if past_values %}
Here are the past iterations of this variable:
<PAST_ITERATIONS>
{{past_values}}
</PAST_ITERATIONS>
Similar feedbacks across different steps suggests that the modifications to the variable are insufficient.
If this is the case, please make more significant changes to the variable.
{% endif %}
{# Constraints #}
{% if constraint_text %}
You must follow the following constraints:
<CONSTRAINTS>{{constraint_text}}</CONSTRAINTS>
{% endif %}
{# In-context examples #}
{% if in_context_examples %}
You must base on the following examples when modifying the {{variable_desc}}:
<EXAMPLES>{{in_context_examples}}</EXAMPLES>
{% endif %}
<END_OF_USER_MESSAGE>
"""

%
OPTIMIZER_SYSTEM_PROMPT = r"""
You are part of an optimization system that refines existing variable values based on feedback.

Your task: Propose a new variable value in response to the feedback.
1. Address the concerns raised in the feedback while preserving positive aspects.
2. Observe past performance patterns when provided and to keep the good quality.
3. Consider the variable in the context of its peers if provided.
   FYI:
   - If a peer will be optimized itself, do not overlap with its scope.
   - Otherwise, you can overlap if it is necessary to address the feedback.

Output:
Provide only the new variable value between {{new_variable_start_tag}} and {{new_variable_end_tag}} tags.

Tips:
1. Eliminate unnecessary words or phrases.
2. Add new elements to address specific feedback.
3. Be creative and present the variable differently.
{% if instruction_to_optimizer %}
4. {{instruction_to_optimizer}}
{% endif %}
"""
\end{lstlisting}

% \minisection{Meta prompts used in Generator backward engine}

% \begin{lstlisting}[
%     basicstyle=\ttfamily\small,
%     breaklines=true,
%     language=Python,
%     keywordstyle=\color{blue}\bfseries,
%     stringstyle=\color{orange},
%     commentstyle=\color{green!50!black},
%     frame=single,
%     showstringspaces=false,
%     tabsize=4,
%     numbers=left,
%     numberstyle=\tiny\color{gray}
% ]    
% 'conversation_sec': 
%     "\n\n<START_OF_VARIABLE_DESC>\nGenerator_input_str\n<TYPE> input (The input to the component.) </TYPE>\n
%     <ROLE>  </ROLE>\n<VARIABLE> I have a microwave, a lamp, four cars, a stove, a toaster, and a bed. How many objects do I have? 
%     </VARIABLE>\n
%     <END_OF_VARIABLE_DESC>\n\n\n
    
%     Here is a conversation with a language model (LM):\n\n
%     NAME: Generator_input_str\nThe target variable is used as either input or a task instruction to a language model (LM):\n\n
%     LM_INPUT: {'input_str': 'I have a microwave, a lamp, four cars, a stove, a toaster, and a bed. How many objects do I have?'}\n
%     LM_OUTPUT: To find the total number of objects you have, you simply count each individual item. In this case, you have a microwave,
%      a lamp, four cars, a stove, a toaster, and a bed. Counting each item separately, the total number of objects you have is 6.\n\n
%      Answer: 6\n", 
     
%      'objective_instruction_sec': 
%      '\nThis conversation is part of a larger system. 
%      The <LM_OUTPUT> was later used as Output from (llm) Generator.\n
%      <OBJECTIVE_FUNCTION>\nYour goal is to give feedback to the variable with the LLM_OUTPUT: 
%      1.\n<CONTEXT>\nThe variable is passed to the eval function and compared with a target/ground truth value.\n\n
%      <EVAL_FUNC_DESCRIPTION>: exact_match: 1 if str(y) == str(y_gt) else 0\n<INPUTS>: (y) (role: Output from (llm) Generator),
%       data: To find the total number of objects you have, you simply count each individual item. In this case, you have a microwave,
%        a lamp, four cars, a stove, a toaster, and a bed. Counting each item separately, the total number of objects you have is 6.\n\n
%        Answer: 6, input_to_eval_fn: 6, data_type: <class \'int\'>\n\n(y_gt) (role: ), data: 9, input_to_eval_fn: 9,
%         data_type: <class \'str\'>\n<OUTPUTS/SCORE>: 0.0\n</CONTEXT>\n\n
%         <FEEDBACK>The output "Generator_outputy_pred_1" was obtained by counting the number of individual items listed. 
%         The generator\'s answer is 6, derived from counting a microwave, a lamp, four cars, a stove, a toaster, and a bed. However, 
%         the exact match evaluation score is 0 because the ground truth value provided is 9. The failure here is due to a miscount of 
%         the items; "four cars" should have contributed 4, making the total 9, but the generator incorrectly counted it as 1. 
%         This discrepancy led to the exact match score of 0.</FEEDBACK>\n</OBJECTIVE_FUNCTION>'}, model_kwargs: {}
%     \end{lstlisting}

\minisection{Example real meta prompt}

On object count, without gradient and score for the optimizer:

\begin{lstlisting}[basicstyle=\ttfamily\small, breaklines=true, frame=single]
<START_OF_SYSTEM_PROMPT>

    You are part of an optimization system that refines existing variable based on feedback generated on a batch of input data.
    
    1. Address the concerns raised in the feedback while preserving positive aspects.
    3. Observe past performance patterns when provided and to keep the good quality.
    4. Consider the variable in the context of its peers if provided.
       FYI:
       - If a peer will be optimized itself, do not overlap with its scope.
       - Otherwise, you can overlap if it is necessary to address the feedback.
    
    Your output should be formatted as a standard JSON instance with the following schema:
    ```
    {
        "reasoning": "Why the variable is proposed this way (str) (required)",
        "proposed_variable": "The proposed variable (str) (required)"
    }
    ```
    -Make sure to always enclose the JSON output in triple backticks (```). Please do not add anything other than valid JSON output!
    -Use double quotes for the keys and string values.
    -DO NOT mistaken the "properties" and "type" in the schema as the actual fields in the JSON output.
    -Follow the JSON formatting conventions.
    
    
    Tips:
    1. Eliminate unnecessary words or phrases.
    2. Add new elements to address specific feedback.
    3. Be creative and present the variable differently.
    4. You can try to show examples to see if it helps.
    
    <END_OF_SYSTEM_PROMPT>
    <START_OF_USER_MESSAGE>
    
    <START_OF_HISTORY_PERFORMANCE>
    Here are the best past iterations of this variable along with the validation score.
    1. value: 'You will answer a reasoning question. Begin by listing each item and its count
      clearly. Then, sum the counts for the total. Your final response should follow this
      format: ''The total number of objects is: $VALUE'' where VALUE is a numerical value.'
    eval_score: 0.84
    2. value: 'You will answer a reasoning question. Think step by step. The last line of
      your response should be of the following format: ''Answer: $VALUE'' where VALUE
      is a numerical value.'
    eval_score: 0.76
    IMPORTANT: Your goal is to generate new variable values that score higher than all previous iterations.
    
    Here are the past failed proposals:
    1. value: 'You will answer a reasoning question. Begin by listing each item and its count
      clearly. Then, sum the counts for the total. Your final response should follow this
      format: ''The total number of objects is: $VALUE'' where VALUE is a numerical value.'
    2. value: 'You will answer a reasoning question. Begin by listing each item and its count
      clearly. Then, sum the counts for the total. Your final response should follow this
      format: ''The total number of objects is: $VALUE'' where VALUE is a numerical value.'
    3. value: 'You will answer a reasoning question. Begin by listing each item and its count
      clearly. Then, sum the counts for the total. Your final response should follow this
      format: ''The total number of objects is: $VALUE'' where VALUE is a numerical value.'
    <END_OF_HISTORY_PERFORMANCE>
    Here are the context and feedback for the variable:
    <START_OF_CONTEXT_FEEDBACK>
    Batch size: 3
    
    1.
    <CONTEXT>
    LM_INPUT: {'input_str': 'I have a bed, a fridge, a lamp, a toaster, four chairs, and a table. How many objects do I have?'}
    LM_OUTPUT: Bed: 1
    Fridge: 1
    Lamp: 1
    Toaster: 1
    Chairs: 4
    Table: 1
    
    The total number of objects is: 9</CONTEXT>
    
    
    2.
    <CONTEXT>
    LM_INPUT: {'input_str': 'I have three oranges, a pig, a frog, a cow, three bananas, a nectarine, and a snail. How many animals do I have?'}
    LM_OUTPUT: Oranges: 3
    Pig: 1
    Frog: 1
    Cow: 1
    Bananas: 3
    Nectarine: 1
    Snail: 1
    
    The total number of animals is: 7</CONTEXT>
    
    
    3.
    <CONTEXT>
    LM_INPUT: {'input_str': 'I have two heads of broccoli, an apple, a lettuce head, and two onions. How many vegetables do I have?'}
    LM_OUTPUT: Sure! Here is the list of vegetables and their counts:
    - Broccoli: 2
    - Lettuce: 1
    - Onion: 2
    
    Now, let's sum the counts:
    2 (broccoli) + 1 (lettuce) + 2 (onion) = 5
    
    Therefore, the total number of vegetables is: 5</CONTEXT>
    <END_OF_CONTEXT_FEEDBACK>
    YOU MUST ENSURE the new variable shares the same intent as the original variable.
    You can either rephrase the initial variable, or add more specific instructions based on the feedback.
    You can not change the variable to only fit on one sample if the batch size is larger than 1.
    <END_OF_USER_MESSAGE>
\end{lstlisting}

Example real meta prompt in multi-hop RAG:

The last node:
\begin{lstlisting}[basicstyle=\ttfamily\small, breaklines=true, frame=single]
<START_OF_SYSTEM_PROMPT>

You are part of an optimization system that refines existing variable based on feedback generated on a batch of input data.

1. Address the concerns raised in the feedback while preserving positive aspects.
3. Observe past performance patterns when provided and to keep the good quality.
4. Consider the variable in the context of its peers if provided.
    FYI:
    - If a peer will be optimized itself, do not overlap with its scope.
    - Otherwise, you can overlap if it is necessary to address the feedback.

Your output should be formatted as a standard JSON instance with the following schema:
```
{
    "reasoning": "Why the variable is proposed this way (str) (required)",
    "proposed_variable": "The proposed variable (str) (required)"
}
```
-Make sure to always enclose the JSON output in triple backticks (```). Please do not add anything other than valid JSON output!
-Use double quotes for the keys and string values.
-DO NOT mistaken the "properties" and "type" in the schema as the actual fields in the JSON output.
-Follow the JSON formatting conventions.


Tips:
1. Eliminate unnecessary words or phrases.
2. Add new elements to address specific feedback.
3. Be creative and present the variable differently.

<END_OF_SYSTEM_PROMPT>
<START_OF_USER_MESSAGE>

<START_OF_HISTORY_PERFORMANCE>
Here are the best past iterations of this variable along with the validation score.
1. value: Respond to questions with precise factoid answers that incorporate full names,
    significant identifiers, and context-appropriate phrases. Always include definitive
    articles like 'the' when relevant, and capture complete geographic or contextual
    details, such as 'Greenwich Village, New York City' when applicable. Think step
    by step while constructing your responses.
eval_score: 0.74
2. value: Answer questions with precise factoid responses, including full names, significant
    identifiers (e.g., titles or notable works), and context-appropriate phrases. Prioritize
    context that directly relates to the question to guide to the correct answer. Always
    think step by step.
eval_score: 0.66
3. value: Answer questions with precise factoid responses, ensuring to include definite
    articles and context-appropriate phrases. Include the word 'from' when answering
    timeframes. You will receive context and a question. Think step by step.
eval_score: 0.64
IMPORTANT: Your goal is to generate new variable values that score higher than all previous iterations.
<END_OF_HISTORY_PERFORMANCE>
Here are the context and feedback for the variable:
<START_OF_CONTEXT_FEEDBACK>
Batch size: 2

1.
<CONTEXT>
LM_INPUT: {'question': 'Which writer was from England, Henry Roth or Robert Erskine Childers?', 'context': [RetrieverOutput(doc_indices=[], doc_scores=None, query=['Which writer was from England, Henry Roth or Robert Erskine Childers?', 'Which writer from England, Henry Roth or Robert Erskine Childers?', 'Find the nationality of Robert Erskine Childers and Henry Roth.'], documents=['Robert Erskine Childers | Robert Erskine Childers DSC (25 June 1870 – 24 November 1922), universally known as Erskine Childers, was a British writer, whose works included the influential novel "The Riddle of the Sands", and a Fenian revolutionary who smuggled guns to Ireland in his sailing yacht "Asgard". He was executed by the authorities of the nascent Irish Free State during the Irish Civil War. He was the son of British Orientalist scholar Robert Caesar Childers; the cousin of Hugh Childers and Robert Barton; and the father of the fourth President of Ireland, Erskine Hamilton Childers.', 'Robert Caesar Childers | Robert Caesar Childers (1838 – 25 July 1876) was a British Orientalist scholar, compiler of the first Pāli-English dictionary. Childers was the husband of Anna Barton of Ireland. He was the father of Irish nationalist Robert Erskine Childers and grandfather to the fourth President of Ireland, Erskine Hamilton Childers.', 'Henry Roth | Henry Roth (February 8, 1906 – October 13, 1995) was an American novelist and short story writer.', "Erskine Barton Childers | Erskine Barton Childers (11 March 1929 – 25 August 1996) was an Irish writer, BBC correspondent and United Nations senior civil servant. He was the eldest son of Erskine Hamilton Childers (Ireland's fourth President) and Ruth Ellen Dow Childers. His grandparents Mary Alden Childers and Robert Erskine Childers and the latter's double first cousin Robert Barton were all Irish nationalists involved heavily with the negotiation of Irish independence; which ultimately led to his grandfather's execution during the Irish Civil War. His great aunt was Gretchen Osgood Warren."])]}
LM_OUTPUT: ```
{
    "reasoning": "Robert Erskine Childers was the writer from England, as he was born in England and was a British writer.",
    "answer": "Robert Erskine Childers was from England."
}
```</CONTEXT>

<FEEDBACK>The current output lacks essential identifiers that would align it with the ground truth. To improve the score on your evaluation function, include significant details such as "DSC" (the designation associated with Robert Erskine Childers) directly in the response. This would create a stronger connection to the original context, thus enhancing your ability to achieve a successful fuzzy match. Additionally, consider reiterating the important context that he was both a British writer and historical figure, as this could provide a richer response. By incorporating these elements step by step into your response, you can ensure that key contextual details are captured effectively.</FEEDBACK>

2.
<CONTEXT>
LM_OUTPUT: ```
{
    "reasoning": "Janet Waldo portrayed Corliss Archer in the film 'Kiss and Tell'.",
    "answer": "The government position held by Janet Waldo, who portrayed Corliss Archer in the film 'Kiss and Tell', was the title character in 'Meet Corliss Archer' on radio."
}
```</CONTEXT>

<FEEDBACK>The response generated by the language model did not directly address the question regarding the specific government position held by Janet Waldo. Instead, it provided information about her character portrayal, which deviates from the core objective. 

To improve alignment with the objective, revise <VARIABLE> to guide the model to focus on pinpointing direct answers to questions about government positions. Emphasizing the need for the inclusion of precise titles or roles, like 'Chief of Protocol', will ensure the model captures essential details from the query. Additionally, instructing the model to extract relevant identifiers related to government positions from the context will help strengthen the accuracy of the responses in future iterations.</FEEDBACK>
<END_OF_CONTEXT_FEEDBACK>
YOU MUST ENSURE the new variable shares the same intent as the original variable.
You can either rephrase the initial variable, or add more specific instructions based on the feedback.
You can not change the variable to only fit on one sample if the batch size is larger than 1.
<END_OF_USER_MESSAGE>
\end{lstlisting}

The second last generator as retriever in the multi-hop RAG:

\begin{lstlisting}[basicstyle=\ttfamily\small, breaklines=true, frame=single]
    <START_OF_SYSTEM_PROMPT>

    You are part of an optimization system that refines existing variable based on feedback generated on a batch of input data.
    
    1. Address the concerns raised in the feedback while preserving positive aspects.
    3. Observe past performance patterns when provided and to keep the good quality.
    4. Consider the variable in the context of its peers if provided.
       FYI:
       - If a peer will be optimized itself, do not overlap with its scope.
       - Otherwise, you can overlap if it is necessary to address the feedback.
    
    Your output should be formatted as a standard JSON instance with the following schema:
    ```
    {
        "reasoning": "Why the variable is proposed this way (str) (required)",
        "proposed_variable": "The proposed variable (str) (required)"
    }
    ```
    -Make sure to always enclose the JSON output in triple backticks (```). Please do not add anything other than valid JSON output!
    -Use double quotes for the keys and string values.
    -DO NOT mistaken the "properties" and "type" in the schema as the actual fields in the JSON output.
    -Follow the JSON formatting conventions.
    
    
    Tips:
    1. Eliminate unnecessary words or phrases.
    2. Add new elements to address specific feedback.
    3. Be creative and present the variable differently.
    
    <END_OF_SYSTEM_PROMPT>
    <START_OF_USER_MESSAGE>
    
    <START_OF_HISTORY_PERFORMANCE>
    Here are the best past iterations of this variable along with the validation score.
    1. value: Construct a detailed search query that interlinks the focal point of the question
      with specific contextual elements, ensuring to specify relevant timeframes and associations
      for comprehensive answers. For instance, inquiring about the director of a film,
      include their projects and significance within their active timeframe, or when exploring
      conference affiliations, explicitly mention historical name changes and their context
      during the years the team was engaged.
    eval_score: 0.74
    2. value: Formulate a focused search query that incorporates relevant timeframes and
      connections for complex questions based on the provided context. For example, ask
      for the screenwriter with credits for 'Evolution' who also co-wrote 'The Family
      Man' during its production period or inquire about the national affiliations of
      Robert Erskine Childers and Henry Ling Roth during their active literary careers.
    eval_score: 0.66
    3. value: Formulate a search query that specifies the relevant details and timeframe
      needed to accurately answer complex questions based on the provided context. For
      example, use 'What was the timeframe for the Manchester United manager who recruited
      David Beckham, specifically during the tenures of Alex Ferguson and Matt Busby?'
      or 'What was the previous name of the America East Conference between 1988 and 1996?'
    eval_score: 0.64
    IMPORTANT: Your goal is to generate new variable values that score higher than all previous iterations.
    <END_OF_HISTORY_PERFORMANCE>
    Here are the context and feedback for the variable:
    <START_OF_CONTEXT_FEEDBACK>
    Batch size: 2
    
    1.
    <CONTEXT>
    LM_INPUT: {'context': ['Robert Erskine Childers | Robert Erskine Childers DSC (25 June 1870 – 24 November 1922), universally known as Erskine Childers, was a British writer, whose works included the influential novel "The Riddle of the Sands", and a Fenian revolutionary who smuggled guns to Ireland in his sailing yacht "Asgard". He was executed by the authorities of the nascent Irish Free State during the Irish Civil War. He was the son of British Orientalist scholar Robert Caesar Childers; the cousin of Hugh Childers and Robert Barton; and the father of the fourth President of Ireland, Erskine Hamilton Childers.', 'Robert Caesar Childers | Robert Caesar Childers (1838 – 25 July 1876) was a British Orientalist scholar, compiler of the first Pāli-English dictionary. Childers was the husband of Anna Barton of Ireland. He was the father of Irish nationalist Robert Erskine Childers and grandfather to the fourth President of Ireland, Erskine Hamilton Childers.', 'Henry Roth | Henry Roth (February 8, 1906 – October 13, 1995) was an American novelist and short story writer.'], 'question': 'Which writer was from England, Henry Roth or Robert Erskine Childers?'}
    LM_OUTPUT: ```
    {
        "reasoning": "To determine the nationality of the writers, we need to focus on their background and origins.",
        "query": "Find the nationality of Robert Erskine Childers and Henry Roth."
    }
    ```</CONTEXT>
    
    <FEEDBACK>To enhance the effectiveness of the constructed search query, consider incorporating additional contextual elements that directly relate to the task at hand. Since the query aims to ascertain the nationality of the writers, specifying details such as their key works, historical significance, and any relevant timelines of their lives would provide a richer context for the language model to retrieve more precise answers. 
    
    For instance, including inquiries that ask about the notable contributions of Robert Erskine Childers to British literature or the impact of Henry Roth's writing in the American literary canon can yield more nuanced results. Additionally, mentioning how their backgrounds influenced their writings might aid in drawing clearer distinctions between them.
    
    Expanding the query to reflect these contextual associations can improve the overall quality and specificity of the answers generated.</FEEDBACK>
    
    2.
    <CONTEXT>
    LM_INPUT: {'context': ["Kiss and Tell (1945 film) | Kiss and Tell is a 1945 American comedy film starring then 17-year-old Shirley Temple as Corliss Archer. In the film, two teenage girls cause their respective parents much concern when they start to become interested in boys. The parents' bickering about which girl is the worse influence causes more problems than it solves.", 'A Kiss for Corliss | A Kiss for Corliss is a 1949 American comedy film directed by Richard Wallace and written by Howard Dimsdale. It stars Shirley Temple in her final starring role as well as her final film appearance. It is a sequel to the 1945 film "Kiss and Tell". "A Kiss for Corliss" was retitled "Almost a Bride" before release and this title appears in the title sequence. The film was released on November 25, 1949, by United Artists.', 'Janet Waldo | Janet Marie Waldo (February 4, 1920 – June 12, 2016) was an American radio and voice actress. She is best known in animation for voicing Judy Jetson, Nancy in "Shazzan", Penelope Pitstop, and Josie in "Josie and the Pussycats", and on radio as the title character in "Meet Corliss Archer".'], 'question': 'What government position was held by the woman who portrayed Corliss Archer in the film Kiss and Tell?'}
    LM_OUTPUT: ```
    {
        "reasoning": "The query aims to find the government position held by the woman who portrayed Corliss Archer in the film 'Kiss and Tell'. To do this, we need to extract information about the actress who played Corliss Archer in 'Kiss and Tell' and her government position.",
        "query": "Janet Waldo government position"
    }
    ```</CONTEXT>
    
    <FEEDBACK>The task description for the query generation should explicitly incorporate contextual elements from both films and the actress's background to enhance the query's focus. Including specific associations, such as the timeline of Janet Waldo's career and notable roles, would likely improve the precision of information retrieval. Additionally, mentioning her prominent role in "Meet Corliss Archer" could provide essential context regarding her significance and potential government involvement. Making these connections can lead to a more comprehensive understanding of Waldo's impact and any related government position, thereby improving the overall objective of the inquiry.</FEEDBACK>
    <END_OF_CONTEXT_FEEDBACK>
    YOU MUST ENSURE the new variable shares the same intent as the original variable.
    You can either rephrase the initial variable, or add more specific instructions based on the feedback.
    You can not change the variable to only fit on one sample if the batch size is larger than 1.
    <END_OF_USER_MESSAGE>
\end{lstlisting}

The first generator as retriever in the multi-hop RAG:

\begin{lstlisting}[basicstyle=\ttfamily\small, breaklines=true, frame=single]
    <START_OF_SYSTEM_PROMPT>

    You are part of an optimization system that refines existing variable based on feedback generated on a batch of input data.
    
    1. Address the concerns raised in the feedback while preserving positive aspects.
    3. Observe past performance patterns when provided and to keep the good quality.
    4. Consider the variable in the context of its peers if provided.
       FYI:
       - If a peer will be optimized itself, do not overlap with its scope.
       - Otherwise, you can overlap if it is necessary to address the feedback.
    
    Your output should be formatted as a standard JSON instance with the following schema:
    ```
    {
        "reasoning": "Why the variable is proposed this way (str) (required)",
        "proposed_variable": "The proposed variable (str) (required)"
    }
    ```
    -Make sure to always enclose the JSON output in triple backticks (```). Please do not add anything other than valid JSON output!
    -Use double quotes for the keys and string values.
    -DO NOT mistaken the "properties" and "type" in the schema as the actual fields in the JSON output.
    -Follow the JSON formatting conventions.
    
    
    Tips:
    1. Eliminate unnecessary words or phrases.
    2. Add new elements to address specific feedback.
    3. Be creative and present the variable differently.
    
    <END_OF_SYSTEM_PROMPT>
    <START_OF_USER_MESSAGE>
    
    <START_OF_HISTORY_PERFORMANCE>
    Here are the best past iterations of this variable along with the validation score.
    1. value: "```\n{\n    \"reasoning\": \"To enhance the effectiveness of the search query,\
      \ it is essential to integrate specific timeframe references, key identifiers, and\
      \ additional contextual elements from the question to guide the search more effectively.\
      \ This revised approach will direct the search toward contextually relevant results,\
      \ which is crucial for accurately answering complex questions. By incorporating\
      \ detailed identifiers, such as release years or names of leagues, the search will\
      \ be more focused, improving the overall search accuracy and relevance.\",\n   \
      \ \"proposed_variable\": \"Generate a detailed search query for a complex question,\
      \ ensuring to integrate specific timeframe references, key identifiers, and contextual\
      \ elements. For instance, include phrases like 'director of the romantic comedy\
      \ \"Big Stone Gap\" released in 2014' or 'Vermont Catamounts men's soccer team America\
      \ East Conference from 1988 to 1996' to facilitate more precise and contextually\
      \ relevant searches.\"\n}\n```"
    eval_score: 0.74
    2. value: Generate a focused search query for a complex question that integrates specific
      timeframe references and key identifiers from the context. For example, include
      phrases like 'screenwriter from the early 2000s who co-wrote a comedy film with
      Nicolas Cage' or '20th-century British authors' to direct the search towards precise
      and contextually relevant results.
    eval_score: 0.66
    3. value: Formulate a concise search query for a complex question by emphasizing temporal
      elements and key identifiers from the given context. For instance, include phrases
      like 'timeframe of management' or 'conference name' directly in the query to guide
      the search towards specific answers.
    eval_score: 0.64
    IMPORTANT: Your goal is to generate new variable values that score higher than all previous iterations.
    <END_OF_HISTORY_PERFORMANCE>
    Here are the context and feedback for the variable:
    <START_OF_CONTEXT_FEEDBACK>
    Batch size: 2
    
    1.
    <CONTEXT>
    LM_INPUT: {'context': [], 'question': 'Which writer was from England, Henry Roth or Robert Erskine Childers?'}
    LM_OUTPUT: ```
    {
        "reasoning": "To enhance the effectiveness of the search query, it is essential to integrate specific timeframe references, key identifiers, and additional contextual elements from the question to guide the search more effectively. This revised approach will direct the search toward contextually relevant results, which is crucial for accurately answering complex questions. By incorporating detailed identifiers, such as release years or names of leagues, the search will be more focused, improving the overall search accuracy and relevance.",
        "query": "Which writer from England, Henry Roth or Robert Erskine Childers?"
    }
    ```</CONTEXT>
    
    <FEEDBACK>To improve the objective function related to the search query generation, consider emphasizing the inclusion of explicit temporal or biographical details that distinctly differentiate the two writers in question. For instance, integrating specific historical contexts or key events associated with Henry Roth and Robert Erskine Childers could significantly refine the search query. 
    
    In your reasoning, rather than solely focusing on general context, explicitly mention the importance of including differentiators such as their most notable works or the time periods they were active. Including phrases like "Henry Roth, known for his novel 'Call It Sleep' published in 1934" or "Robert Erskine Childers, a notable figure during the Irish War of Independence" can enhance the specificity and relevance of the search results, leading to a more effective inquiry into the question posed.
    
    By revising the proposed variable to emphasize these unique identifiers, the query will likely yield more accurate and relevant information, thereby improving the overall search effectiveness.</FEEDBACK>
    
    2.
    <CONTEXT>
    LM_INPUT: {'context': [], 'question': 'What government position was held by the woman who portrayed Corliss Archer in the film Kiss and Tell?'}
    LM_OUTPUT: ```
    {
        "reasoning": "To enhance the effectiveness of the search query, it is essential to integrate specific timeframe references, key identifiers, and additional contextual elements from the question to guide the search more effectively. This revised approach will direct the search toward contextually relevant results, which is crucial for accurately answering complex questions. By incorporating detailed identifiers, such as release years or names of leagues, the search will be more focused, improving the overall search accuracy and relevance.",
        "query": "Government position held by the woman who portrayed Corliss Archer in the film Kiss and Tell"
    }
    ```</CONTEXT>
    
    <FEEDBACK>To improve the effectiveness of the search query generated for complex questions, you should emphasize the inclusion of specific identifiers and contextual elements in both the reasoning and proposed outputs. The current reasoning highlights the importance of timeframe references, which is beneficial. However, it lacks concrete examples that align more closely with the user's query.
    
    Consider including more specific suggestions related to the user's context, such as referencing the actress's name alongside her character or film title. For instance, you might state: "A more precise query could be crafted by including the actress's name and the film's release year." This clarity in your reasoning reinforces the importance of context in generating relevant search queries.
    
    Additionally, the proposed variable could further enrich the search by not only mentioning the movie title but also introducing related terms, such as the actress's name or accolades associated with the film. Doing so will create a more directed search, yielding better results in terms of accuracy and relevancy. 
    
    In summary, strengthen the connection between the details and the expected search outcomes by providing richer examples and focusing on characterizing contextual relevance more clearly in the final query.</FEEDBACK>
    <END_OF_CONTEXT_FEEDBACK>
    YOU MUST ENSURE the new variable shares the same intent as the original variable.
    You can either rephrase the initial variable, or add more specific instructions based on the feedback.
    You can not change the variable to only fit on one sample if the batch size is larger than 1.
    <END_OF_USER_MESSAGE>
    
\end{lstlisting}

\minisection{Example feedback \& context \& value \& new value for prompt parameter}

% One LLM call computation graph 

% \begin{figure}
%     \centering
%     \includegraphics[width=0.8\textwidth]{one_llm_call.png}
%     \caption{LLM call computation graph}
%     \label{fig:llm_call_graph}
% \end{figure}

This shows an object count task with sum operation, batch size 2 with two loss outputs.
Two generator outputs and one system prompt. 
The key parts are the backward engine on the loss component and the backward engine on the generator component.
Eventually an optimizer that aggregates the feedback from the backward engines to propose a new prompt parameter value.

In AdalFlow, the gradient context is tracked as Data Structure \textit{GradientContext} in the backward pass along with the gradients.
In the forward pass, we use similr code to track all context 
\begin{lstlisting} [language=Python, basicstyle=\ttfamily\small, breaklines=true]
    pred.gradients_context[var_gradient] = GradientContext(
            context=conversation_str,
            response_desc=response.role_desc,
            parameter_desc=pred.role_desc,
        )
\end{lstlisting}
The goal is to set the context for predecessor node.

% new table
\begin{table}[ht]
    \centering
    \fontsize{8.5}{10}\selectfont

    \begin{tabular}{l p{8cm} p{4cm} p{3cm}}
        \toprule
        \textbf{Parameter} &   \textbf{Value} &\textbf{GradientContext}          & \textbf{Gradient}     \\
        \midrule
        Question(leaf) & Uyirodu Uyiraga was a film that starred the Indian actor who participated in what 2004 sporting event?               &  &           \\
        \midrule
        GT(leaf)                          & British Formula 3 season&                           \\
        \midrule
        \multirow{2}{*}{Planner Task(prompt)}                          &   You are an excellent task planner. Answer the input query using the tools provided below with maximum accuracy.\n\n Each step you will read the previous thought, Action(name, kwargs), and Observation(execution result of the action) and then provide the next Thought and Action.\n\n\n Follow function docstring to best call the tool.\n- For simple queries: Directly call the 'finish' action and answer with a concise 'yes' or 'no' when it fits.\n- For complex queries:\n    - Step 1: Understand the main subject(s) and context of the user query accurately.\n    - Step 2: Break down the query into multisteps, starting with the first tool/subquery.\n    - Ensure each step accurately reflects the subjects under consideration.\n    - Continuously verify your extracted information and logic for factual accuracy using concise comparisons.\n    - At step 'finish', conclude with a precise final answer.\n REMEMBER:\n- Action MUST call one of the tools. It CANNOT be empty.\n- You will ALWAYS END WITH 'finish' tool to conclude the task directly with an answer or failure message.\n- When the tool is a class method and when class\_instance exists, use . to call instead (NOT the CLASS NAME).
             & \textbf{Skip Connection}
            "variable\_desc": "Task instruction for the agent to plan steps to solve a question in sequential and multi-steps to get the final answer.                 For optimizer: you need to adapt this to the current specific task.",
           "input\_output":"\n COMPONENT\_DESC: Extract the final answer from the step history.\n\nINPUTS:\n1.\nKEY: step\_history\_0.\nROLE: The result of the action execution, observation is the final answer,...                                     \\
        \midrule
        Step 1 LLM output               & "thought": "I need to retrieve information about the film 'Uyirodu Uyiraga' and the Indian actor who starred in it.", "name": "dspy\_retriever\_as\_tool",
        "args": [],
        "kwargs": {
            "input": "Uyirodu Uyiraga Indian actor 2004 sporting event",
        }&   &\\
        Step 1 Execution Result              & 
        \textbf{"observation": [
        "Uyirodu Uyiraga | Uyirodu Uyiraga is a 1998 Tamil film directed by Sushma Ahuja starring Ajith Kumar and Richa Ahuja in the main roles. The film which told the tale of a couple's struggle to deal with terminal illness, had a successful music soundtrack composed by Vidyasagar. The film was released in November 1998 to positive reviews, but fared poorly commercially.",
        "K. M. Binu | Kalayathumkuzhi Mathews Binu (born 20 December 1980) is an Indian track and field athlete from Kerala who specializes in 400 metres and 800 metres. He holds the current 400 metres national record of 45.48 s set at the 2004 Athens Olympics on 20 August 2004. He broke the 44-year-old Olympics mark (by an Indian) held by Milkha Singh who set an Indian National Record with a timing of 45.73 s at the 1960 Rome Olympics. He and his elder sister K. M. Beenamol made history when they became the first Indian siblings to win medals in a major international competition. They won medals at the Busan Asian Games (2002). While Binu won the men's 800 metres silver, his sister won the gold medal in the women's event. Binu received the Arjuna Award for the year 2006 for his achievements in the Indian athletics."
    ]} \\
        Step 2 LLM output       &   {
        "thought": "The retrieved information does not mention the Indian actor who participated in the 2004 sporting event. I need to retrieve more specific details.",
        "name": "dspy\_retriever\_as\_tool",
        "args": [],
        "kwargs": {
            "input": "Uyirodu Uyiraga 2004 Indian actor sporting event",
        }
    }                        &                                \\
        Agentic RAG                &                                                         \\

        \bottomrule
    \end{tabular}
    \caption{Demonstration of gradients in React's auto-differentiable Graph.}
    \label{tab:agentic_gradients}
\end{table}
